# Supplementary material for: Understanding Diffusion of Recurrent Innovations
Source: arXiv:2101.05094 source file (2021-01-13)
Supplement: Supplementary file 1 [file appendix.tex]

%\section{Prediction of the adoption behaviors of users}
%This section provides details of data pre-processing, feature selection, and results in Section~\ref{sec:regression}.
%
%\subsection{Detailed Pre-processing}
%The detailed data pre-processing procedures can be listed as follows.
%
%First of all, we only select apps with 500 or more users and versions with 100 or more users, in order to reduce noise and filter out test versions. 
%Second, due to the lack of mapping data of app versions to their official release time in app markets because the apps are anonymized, we infer the release time of a version by the time it has the 50th adopter.
%
%With the data processed, we further select app versions to make the prediction feasible. In specific, for each app, we select its first version released in May, 2019 and users with usage logs since April 1st, 2019. In this way 4,955 different versions and 8,248,388 users are selected. Furthermore, because the number of users varies a lot in different versions, we adopt a down-sampling strategy to make each version comparable. Specifically,  we select the 1,651 versions (i.e., 1/3 of all versions) with the most users to balance the number of versions and the users of each version. 
%
%\subsection{Feature Selection}
%
%We cluster the features according to their correlation coefficients and plot the dendrogram, which shows high correlation between some features, most of which are from the same dimension. By selecting one feature from each bunch in which correlation coefficients are higher than 0.7, we have 12 features to feed into the classification models. Similarly, we also have 12 features for the regression models.
%
%\subsection{Results}
%\input{tables/basic-importance-coef}
%
%Table~\ref{table:basic-importance-coef} presents the detailed importance and coefficients of features in the classification of adoption task and regression of adoption task.
%
%\section{Detection of different types of adopters}\label{appendix:types}
%This section provides details of adopter type detection for the analysis in Section~\ref{sec:regression-special}. The detection is based on the dataset selected in Section~\ref{sec:regression}.
%
%\subsection{Subscribers}
%% Before understanding the adoption patterns, we need to recognize the adopters with specific patterns at first. 
%For each version, we set a threshold of the days to adopt and users who adopt this version within the threshold are considered as the subscribers of the version. We find that 76.73\% versions achieves their first peak within 1 day in the incremental adoption curve of their existing adopters. We then set the threshold to be 1 day. In this way, we get 53,858 positive observations, and 168,574 negative observations.
%
%\subsection{Preservers}
%If a target app releases more than one version after 1st May, 2019 and the user adopts only the first one, the user is classified to the preservers. In this way, 75,454 users are recognized as preservers. As for the negative observations, we randomly sample users who adopt more than one versions of target apps. Finally, we get 202,266 observations.
%
%\subsection{Retro-adopters}
%If a user adopt a target version of a specific app and then adopt the previous versions of the same app, they are considered as retro-adopter. We find 19,359 retro-adopters. We randomly sample another group of users, who do not adopt previous versions after adopting the target version, from the same groups of apps as negative observations. In this way, we get 80,000 observations.
